# Supplementary material for: Face Mask Removal with Region-attentive Face Inpainting
Source: arXiv:2409.06845 source file (2025-04-02)
Supplement: Supplementary file 1 [file Supplementary.tex]

\section{Effectiveness of Multi-scale Feature Aggregation Structure}
\label{sec:spp}
In the Multi-scale Channel-Spatial Attention Module (M-CSAM) (shown in \cref{fig:M-CSAM}), we adopt a multi-scale feature aggregation structure to explore features from four different receptive scales. Features obtained with larger receptive fields tend to be more robust to texture and color variation, while features from smaller receptive fields focus more on details. The combination of features from different receptive fields is shown to be effective for masked region recovery as shown in \cref{fig:abs_multiscale} and \cref{table:multi-scale}.

To illustrate the effectiveness of multi-scale structure, we performed an experiment without the multi-scale structure. As shown in \cref{table:multi-scale}, when the multi-scale structure is removed, the performance drops in terms of all metrics, namely SSIM, PSNR and $\ell_1$ loss. \cref{fig:abs_multiscale} provides some examples for qualitative comparison. As can be seen, without multi-scale feature aggregation module, the recovered regions have distorted areas (see \cref{fig:ab3_c} and \cref{fig:ab3_d}). The network equipped with multi-scale feature aggregation module incorporates larger receptive fields and a better semantic understanding. Therefore, with the assistance of the multi-scale feature aggregation module, the recovered content is more consistent with the ground truth, and has better continuity and texture.

\begin{figure}[ht!]
\begin{center}
% \fbox{\rule{0pt}{2in} \rule{0.9\linewidth}{0pt}}
  \includegraphics[width=1\linewidth]{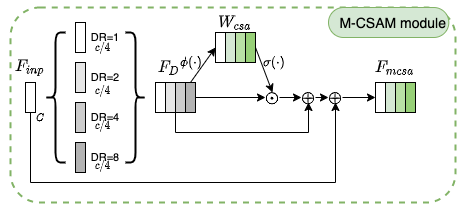}
\end{center}
\vspace{-0.3cm}
  \caption{The structure of M-CSAM.}
\label{fig:M-CSAM}
\end{figure}

\begin{table}[ht!]
\vspace{-0.1cm}
\centering
\scalebox{1}{
\begin{tabular}{ @{}l c c r @{}}
 \hline
 & SSIM$^+$  &  PSNR$^+$  & $\ell_1^-$ loss\\
 \hline
 M-CSAM   & \textbf{0.9511} & \textbf{30.3885} & \textbf{0.0076}\\
 CSAM   & 0.9454  & 29.6126  & 0.0084\\
 \hline
\end{tabular}}
\vspace{-0.2cm}
\caption{The effect of multi-scale feature aggregation structure. $^+$Higher is better. $^-$Lower is better.}
\label{table:multi-scale}
\vspace{-0.2cm}
\end{table}

\begin{figure}[ht!]
\centering
\begin{subfigure}{0.24\linewidth}
        \includegraphics[width=1.0\linewidth]{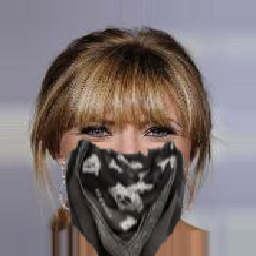}\\
        \includegraphics[width=1.0\linewidth]{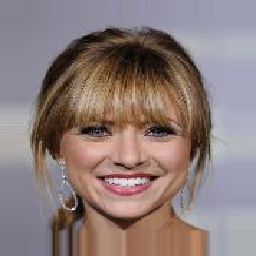}\\
        \includegraphics[width=1.0\linewidth]{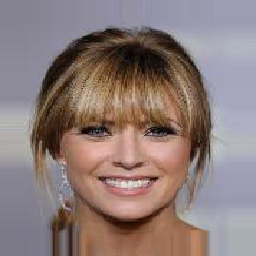}\\
        \includegraphics[width=1.0\linewidth]{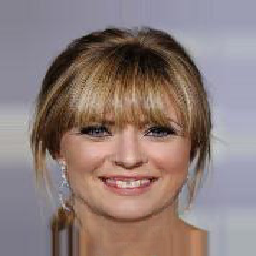}
    \caption{}
    \label{fig:ab3_a}
\end{subfigure}
\begin{subfigure}{0.24\linewidth}
        \includegraphics[width=1.0\linewidth]{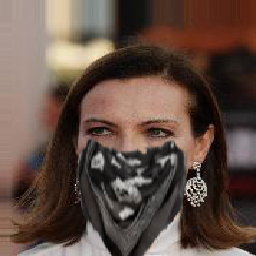}\\
        \includegraphics[width=1.0\linewidth]{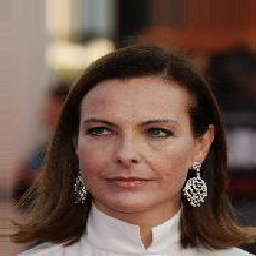}\\
        \includegraphics[width=1.0\linewidth]{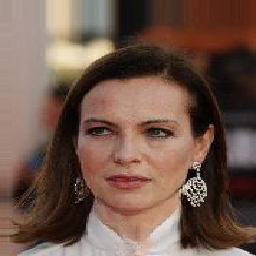}\\
        \includegraphics[width=1.0\linewidth]{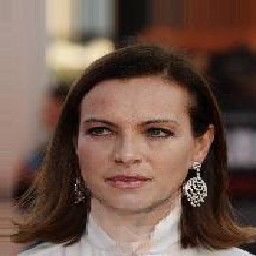}
    \caption{}
    \label{fig:ab3_b}
\end{subfigure}
\begin{subfigure}{0.24\linewidth}
        \includegraphics[width=1.0\linewidth]{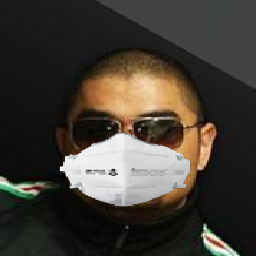}\\
        \includegraphics[width=1.0\linewidth]{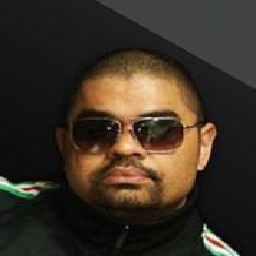}\\
        \includegraphics[width=1.0\linewidth]{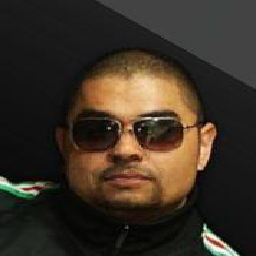}\\
        \includegraphics[width=1.0\linewidth]{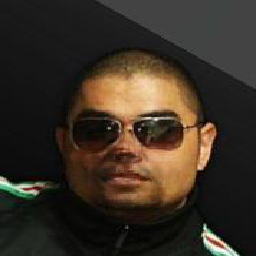}
    \caption{}
    \label{fig:ab3_c}
\end{subfigure}
\begin{subfigure}{0.24\linewidth}
        \includegraphics[width=1.0\linewidth]{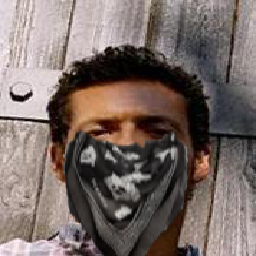}\\
        \includegraphics[width=1.0\linewidth]{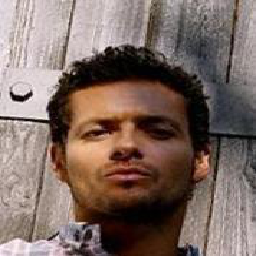}\\
        \includegraphics[width=1.0\linewidth]{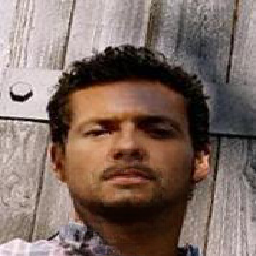}\\
        \includegraphics[width=1.0\linewidth]{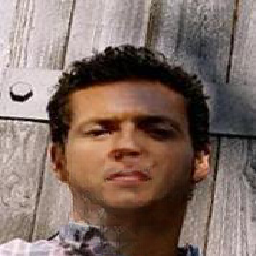}
    \caption{}
    \label{fig:ab3_d}
\end{subfigure}
\vspace{-0.2cm}
\caption{\textbf{Qualitative comparison of models with and without multi-scale feature aggregation structure.} First row: input images with face masks; Second row: ground-truth images; Third row: results from the network with multi-scale feature aggregation structure; Fourth row: results from the network without multi-scale feature aggregation structure (best viewed when zoomed-in).}
\label{fig:abs_multiscale}
\end{figure}
